# Supplementary material for: Beyond Text: Unveiling Multimodal Proficiency of Large Language Models with MultiAPI Benchmark
Source: arXiv:2311.13053 source file (2023-11-21)
Supplement: Supplementary file 1 [file 9-appendix.tex]

\newpage
\section{Domain and Required Arguments Mapping}
\label{app:domian_arg_map}

\section{Dataset Construction Prompts}
\label{app:data_const_prompt}

\section{Experiment Prompts}
\label{app:exp_prompt}
